# Supplementary material for: Towards a certified reference monitor of the Android 10 permission system
Source: arXiv:2011.00720 source file (2020-10-29)
Supplement: Supplementary file 1 [file appendix.tex]

\appendix
\section{Valid state} %\label{app:validstate}

%\subsection*{Valid state} 
\label{app:validstate}
\small
The model formalizes a notion of valid state that captures several well-formedness conditions. It is formally defined as a predicate \textit{valid\_state} on the elements of type $\AndroidState$. This predicate holds on a state $s$ if the following conditions are met: 
%\begin{inparaenum}[i)]
\begin{itemize} 
\item all the components both in installed applications and in system applications have different identifiers;
\item no component belongs to two different applications present in the device;
\item no running component is an instance of a content provider;
\item every temporally delegated permission has been granted to a currently running component and over a content provider present in the system;
\item every running component belongs to an application present in the system;
\item every application that sets a value for a resource is present in the system;
\item the domains of the partial functions $\AppsManifest$, $\AppsCert$ and $\AppsDefPerms$ are exactly the identifiers of the user installed applications;
\item the domains of the partial functions $\AppsPerms$ and $\GrantedGroups$ are exactly the identifiers of the applications in the system, both those installed by the users and the system applications;
\item every installed application has an identifier different to those of the system applications, whose identifiers differ as well;
\item all the permissions defined by applications have different identifiers;
\item every partial function is indeed a function, that is, their domains don't have repeated elements;
\item every individually granted permission is present in the system; and
\item all the sent intents have different identifiers.
\end{itemize}
%\end{inparaenum}

All these safety properties have a straightforward interpretation in our model. We omit here the formal definition of \textit{valid\_state} due to space constraints. The full formal definition of the predicate is available in \cite{AndroidCoq:2016}. %\cite{AndroidCoq:2016}.
%Valid states are invariant under execution, as will be shown later.

%A notion of \emph{valid state}, that captures several well-formedness conditions, is formally defined as a predicate \textit{validState} on the elements of type $\AndroidState$.  For instance, a property states that all the running instances belong to a unique component, which is part of an installed application. %Valid states are invariant under execution.
\normalsize
%\subsection{Actions} 
%\label{app:actions}

\section{Generated code} \label{code}
Just for the sake of illustration, in what follows we provide listings of part of the Haskell code that has been automatically generated using the Coq extraction mechanism. The code is annotated with inline comments and manually indented to fit on the page width. 

We have included the definition of the System, as a datatype and  the complete definition of the action \texttt{install} and the code of the dispatcher,  which implements the execution of an action in a given state.

\newpage

%\lstinputlisting{commented_code.hs}
\begin{lstlisting}[frame=lines,basicstyle=\tiny,caption={The System}, label={lst:system-state}]
{- The System is represented as a datatype
 - comprising a State and an Environment 
 -}

data System =
   Sys State Environment

-- The Environment datatype
data Environment =
   Env
   -- The manifest and certificate of installed user applications 
     (Mapping IdApp Manifest)   
     (Mapping IdApp Cert)
   -- The permissions defined by the applications
     (Mapping IdApp (([]) Perm0))  
   -- System applications
     (([]) SysImgApp)                      

-- The datatype State
data State =
   St 
   -- The installed user applications 
     (([]) IdApp)  
   -- Granted group and individual permissions for each application 
     (Mapping IdApp (([]) IdGrp)) 
     (Mapping IdApp (([]) Perm0))
   -- Running components and their instances
     (Mapping ICmp Cmp)    
   -- Permanent and temporary permission delegations
     (Mapping ((,) ((,) IdApp CProvider) Uri) PType)  
     (Mapping ((,) ((,) ICmp CProvider) Uri) PType)
   -- Values of resources
     (Mapping ((,) IdApp Res) Val) 
   -- Sent intents
     (([]) ((,) ICmp Intent0)) 
\end{lstlisting}

\begin{lstlisting}[frame=lines,basicstyle=\tiny,caption={Install checks}, label={lst:installprec}]
{- Install semantics:
 - install_pre checks whether an installation can take place in a state.
 - It returns the corresponding ErrorCode if the installation is not allowed
 -}

install_pre :: IdApp -> Manifest -> Cert -> (([]) Res) ->
    System -> Prelude.Maybe ErrorCode
install_pre app0 m c lRes s =
-- The application can not be already installed
  case isAppInstalledBool app0 s of {
   Prelude.True -> Prelude.Just App_already_installed;
   Prelude.False ->
-- Components in the application must have different identifiers
    case has_duplicates idCmp_eq (map getCmpId (cmp m)) of {
     Prelude.True -> Prelude.Just Duplicated_cmp_id;
     Prelude.False ->
-- The defined permissions must have different identifiers.
      case has_duplicates idPerm_eq (map idP (usrP m)) of {
       Prelude.True -> Prelude.Just Duplicated_perm_id;
       Prelude.False ->
-- The new components' ids must differ from those already present in the system.
        case existsb (\c0 -> cmpIdInStateBool c0 s) (cmp m)
        of {
         Prelude.True -> Prelude.Just Cmp_already_defined;
         Prelude.False ->
-- No permission defined by other application can be redefined.
          case Prelude.not (authPermsBool m s) of {
           Prelude.True -> Prelude.Just
           Perm_already_defined;
           Prelude.False ->
-- All the intent filters must be well defined.
            case anyDefinesIntentFilterIncorrectly (cmp m)
            of {
             Prelude.True -> Prelude.Just
                Faulty_intent_filter;
-- If everything is ok, then no error is returned.
             Prelude.False -> Prelude.Nothing}}}}}}
\end{lstlisting}

\newpage

\begin{lstlisting}[frame=lines,basicstyle=\tiny,caption={Install effect}, label={lst:installpost}]
{- The function install_post compute the state resulting from 
 - installing a fresh application
 -}

install_post :: IdApp -> Manifest -> Cert -> (([]) Res) ->
    System -> System
install_post app0 m c lRes s =
  let {oldstate = state s} in
  let {oldenv = environment s} in
-- The application identifier is appended to the list of installed applications
  Sys (St ((:) app0 (apps oldstate))
-- with no permission or permission groups granted,
  (map_add idApp_eq (grantedPermGroups oldstate) app0 ([]))
  (map_add idApp_eq (perms oldstate) app0 ([])) (running
  oldstate)
  (delPPerms oldstate) (delTPerms oldstate)
-- its resources are initialized with the default value, and
  (addNewResCont app0 (resCont oldstate) lRes) (sentIntents
  oldstate))
-- its manifest, certificate and permissions are stored in the state.
  (Env
  (map_add idApp_eq (manifest oldenv) app0 m)
  (map_add idApp_eq (cert oldenv) app0 c)
  (map_add idApp_eq (defPerms oldenv) app0 (nonSystemUsrP m))
  (systemImage oldenv))
\end{lstlisting}

\begin{lstlisting}[frame=lines,basicstyle=\tiny,caption={Safe install}, label={lst:safeinstall}]
{- The function install_safe checks for errors using the function install_pre,
 - returning the state unmodified along with the error code, if there is one.  
 - Otherwise, it computes the new state by executing install_post
 -}

install_safe :: IdApp -> Manifest -> Cert -> (([]) Res) -> System -> Result0
install_safe app0 m c lRes s =
  case install_pre app0 m c lRes s of {
   Prelude.Just ec -> Result (Error0 ec) s;
   Prelude.Nothing -> Result Ok (install_post app0 m c lRess)}
\end{lstlisting}

\begin{lstlisting}[frame=lines,basicstyle=\tiny,caption={Dispatcher}, label={lst:dispatcher}]
{- The function step is just a dispatcher which
 - performs pattern matching on the action to be
 - executed and calls the corresponding function
 - (for example, install_safe)
 -}

step :: System -> Action -> Result0
step s a =
  case a of {
   Install app0 m c lRes -> install_safe app0 m c lRes s;
   Uninstall app0 -> uninstall_safe app0 s;
   Grant p app0 -> grant_safe p app0 s;
   Revoke p app0 -> revoke_safe p app0 s;
   GrantPermGroup grp app0 -> grantgroup_safe grp app0 s;
   RevokePermGroup grp app0 -> revokegroup_safe grp app0 s;
   HasPermission a0 p -> Result Ok s;
   Read0 ic cp u -> read_safe ic cp u s;
   Write0 ic cp u v -> write_safe ic cp u v s;
   StartActivity intt ic -> startActivity_safe intt ic s;
   StartActivityForResult intt n ic -> startActivity_safe intt ic s;
   StartService intt ic -> startService_safe intt ic s;
   SendBroadcast intt ic p -> sendBroadcast_safe intt ic p s;
   SendOrderedBroadcast intt ic p -> sendBroadcast_safe intt ic p s;
   SendStickyBroadcast intt ic -> sendStickyBroadcast_safe intt ic s;
   ResolveIntent intt a0 -> resolveIntent_safe intt a0 s;
   ReceiveIntent intt ic a0 -> receiveIntent_safe intt ic a0 s;
   Stop ic -> stop_safe ic s;
   GrantP ic cp a0 u pt -> grantP_safe ic cp a0 u pt s;
   RevokeDel ic cp u pt -> revokeDel_safe ic cp u pt s;
   Call ic sac -> call_safe ic sac s }
\end{lstlisting}

\newpage
\section{Answers to reviews}
\input{answers-lopstr.txt}
